# Supplementary material for: Cross-Modal Retrieval Meets Inference:Improving Zero-Shot Classification with Cross-Modal Retrieval
Source: arXiv:2308.15273 source file (2023-08-29)
Supplement: Supplementary file 1 [file appendix.tex]

\appendix

\section{Reproducibility}
The code for experiments in this paper can be found here: \url{https://anonymous.4open.science/r/X-MoRe-1DC0}. The retrieved captions for partial datasets are available in the supplemental materials. The retrieval module of our method is based on an open source code from clip-retrieval\footnote{https://github.com/rom1504/clip-retrieval} which implements KNN retrieval based on autofaiss\footnote{https://github.com/facebookresearch/faiss}. The setting of the retrieval module can be found at clip-retrieval and we provide configuration file which is included in supplemental materials.
For every evaluation on each dataset, we use a single RTX A5000 GPU with 24GB memory.

\section{Inference Budget}
We include a comparison of inference budgets for training and inference methods of CLIP in Table \ref{tab:budget}. While the major computation overhead of prompt tuning based methods comes from the 1-step optimization which involves back propagations through the text encoder of CLIP and linearly scales to number of categories when forwarding class texts with templates, e.g., ``a photo of a [CLS],'' our method does not depend on them.

Despite the inference speed of one of our baseline, CALIP \cite{guo2023calip} is same as that of CoOp or CLIP with hand-crafted prompts, additional inference cost exists when searching for logit weights in grid manner for weighted sum.

We also report that the retrieval cost of \texttt{X-MoRe} is 30 $\sim$ 40ms per one nearest-neighbor retrieval of candidate image-caption pairs in 100GB sized indices of laion-4oom dataset where the number of retrieved neighbor is 200.

\begin{table*}[t!]
    \begin{tabular}{lccccc}
    \toprule
    & Hand-crafted & CoOp  & TPT & CALIP & X-MoRe\\
    & \footnotesize\cite{radford2021learning} & \footnotesize\cite{zhou2022learning} & \footnotesize\cite{guo2023calip} & \footnotesize\cite{shu2022test} & \footnotesize(Ours) \\
    % & \scriptsize\cite{radford2021learning} & \scriptsize\cite{zhou2022learning} & \scriptsize\cite{zhou2022conditional} & \scriptsize\cite{shu2022test} & \scriptsize(Ours) \\
    \midrule
    Inference speed (seconds/iter) & 0.002 & 0.002 & 0.16 & 0.002 & 0.02 \\
    Number of training samples & 0 & 16K & 0 & 0 & 0 \\
    % Number of additional parameters & 0 & 0 & 65.8K & 0 & 0 \\
    % Natural language prompt$\textsuperscript{†}$ & \cmark & \xmark & \xmark & \cmark & \cmark \\
    Prompt tuning & \xmark & \cmark & \cmark & \xmark & \xmark \\
    Number of training parameters & 0 & 2K & 2K & 0 & 0 \\
    \bottomrule
    \end{tabular}
    \centering
    \caption{Comparison of training and testing budgets of prompting strategies for CLIP. Natural language prompt$\textsuperscript{†}$ refers to the use of the discrete embeddings of the phrase ``a photo of a [CLS]'' without prompt tuning.}
    \label{tab:budget}
\end{table*}

\section{Retrieval Examples}
%\subsection{Visualization}
% input image, retrieved captions
% 이미지 기반으로 했을때 결과.
% 텍스트 기반으롷 해쓸 떄 결과
% 최종까지 (3단계로)
%자리 남으면 main에 넣고 안되면 appendix 맨위에라도 해서, main에서 pointing
We present the visualization results of Section 3.2 Cross-modal Retrieval. The method contains coarse-level retrieval based on image modality and a following fine-level retrieval based on text modality, as shown in Figure \ref{fig:appendix_viz}. Captions which correspond to image input from fine-grained datasets, such as Flower102, Pets, Food101, Cars, or FGVCAircraft often contain precise words referring to object in an image; for example, ``Sweet William'' in Flower102 or ``Ford Mustang'' in Cars. In other cases, captions contain expressions which illustrate the image in general. For instance, ``View of a River'' or ``Highways intersecting'' in captions from SUN397 and EuroSAT respectively, describe the landscape contained in each image. 

This observation that certain precise words or semantically close synonyms to certain categories are involved in retrieved captions also support our analysis in Section 6.1 on the entropy comparison when using single caption compared to that of using single image. Previously mentioned in the analysis, this justifies our method using caption ensemble which alleviates the low entropy in contrast to lower accuracy than image modality, since this unique characteristic of caption retrieval may contain overconfident incorrect predictions.

As shown in the examples in Figure \ref{fig:appendix_viz}, fine-retrieval is the key step for retrieving accurate captions, presenting in visible proofs that ranking of captions from image-based retrieval do not align with that from direct similarity between the query image and captions. 
%Further analysis is in Appendix on ranking correlation.

\begin{figure*}[t!]
    \centering
    \includegraphics[width=\textwidth]{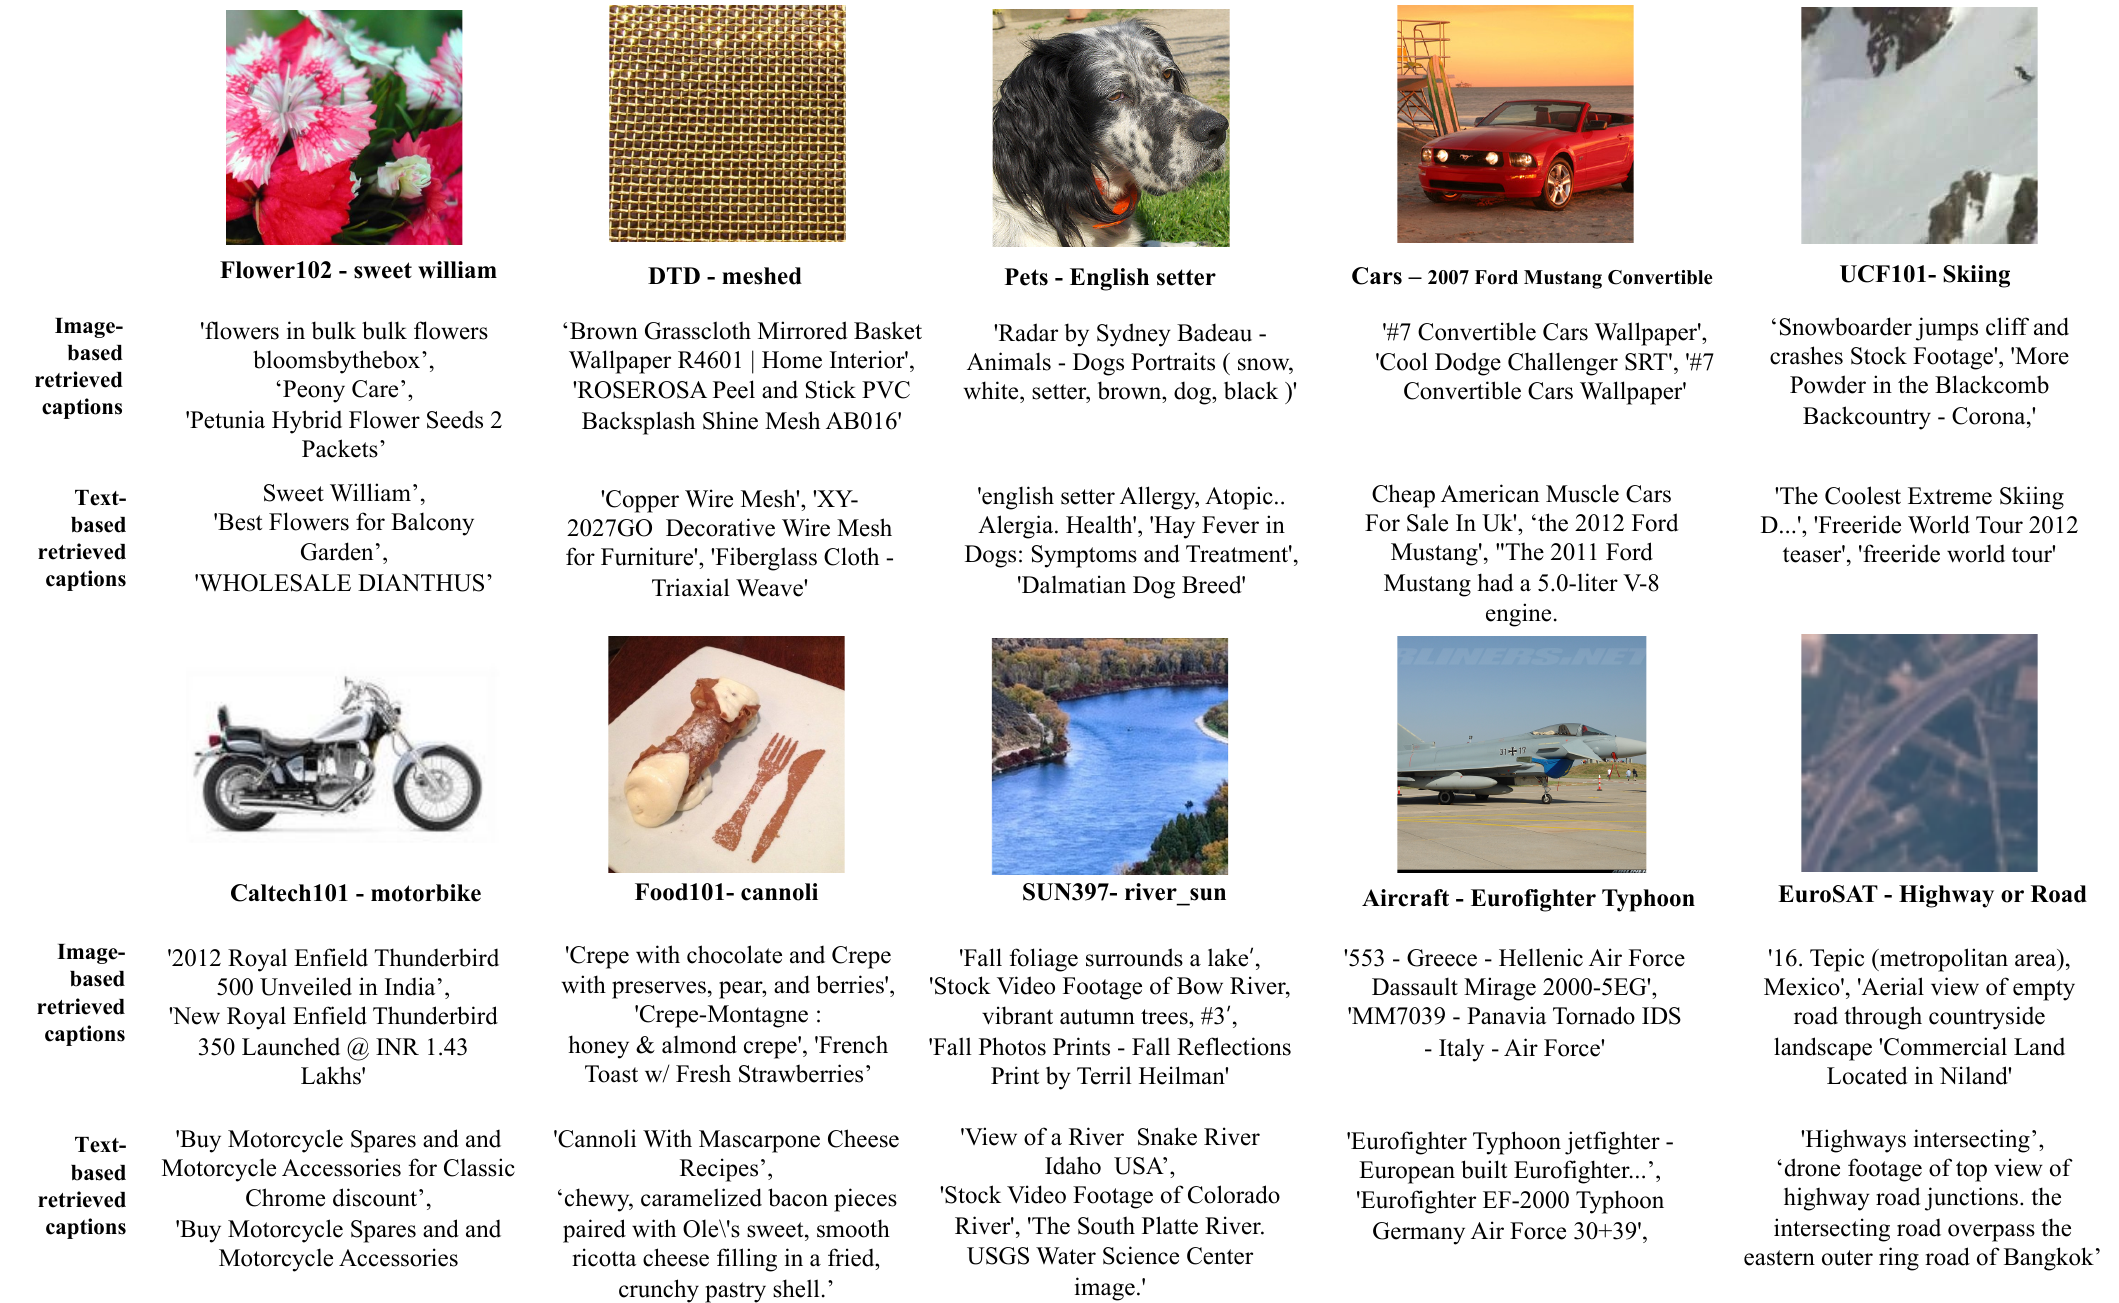}
    \caption{Retrieved captions of each sample from 10 image classification datasets (`dataset' - `label text'). Two retrieved caption sets are intermediate and final results from cross-modal retrieval, i.e., image-based retrieval and text-based retrieval. Compared to image-based retrieved captions, text-based retrieved captions are more accurate and better describe input sample.}
    \label{fig:appendix_viz}
\end{figure*}

\section{Experiments}
\subsection{Effect of the Number of Retrieved Captions}
For Table \ref{tab:appendix_variousK_finegrained} and \ref{tab:appendix_variousK_imagenet}, we report detailed evaluation results of our method. Examining the results, retrieving more captions does not help improving the performance, indicating that retrieving fine quality captions is more crucial than using many captions. For most of cases aside from using CLIP-VIT-B/16 in imagenet variants, our method exceed tuning-based inference method, i.e. TPT. In relation to performance gain, our method delivers a notable boost when both modalities show similar results. Yet, when the performance discrepency exists between the two modalities, i.e., `CLIP-ViT-B/16' and `Caption Ensemble,' our method lags behind. 

\begin{table*}[h]
\small
\centering
\setlength{\tabcolsep}{3pt}
    \begin{tabular}{l|cccccccccc|c}
    \toprule
    Method & Flower102 & DTD & Pets & Cars & UCF101 & Caltech101 & Food101 & SUN397 & Aircraft & EuroSAT & Avg. \\
    \midrule
    CLIP-RN50$^{\dagger}$ & 61.75 & 40.37 & 83.57 & 55.70 & 58.84 & 85.88 & 73.97 & 58.80 & 15.66 & 23.69 & 55.82 \\
    Caption Ensemble & 59.36 & 35.40 & 62.74 & 43.82 & 51.44 & 81.82 & 70.00 & 49.44 & 19.50 & 29.65 & 50.32 \\
    CALIP & 60.90 & 39.89 & 81.25 & 55.64 & 54.59 & 83.94 & 71.49 & 56.84 & 15.72 & 24.22 & 54.45\\
    TPT$^{\dagger}$ & 62.69 & 40.84 & 84.49 & 58.46 & 60.82 & 87.02 & 74.88 & 61.46 & 17.58 & 28.33 & 57.66 \\
    X-MoRe ($K$=2) & 65.98 & 44.29 & 79.71 & 55.44 & 64.21 & 88.87 & 79.07 & 60.22 & 18.99 & 30.91 & 58.77 \\
    X-MoRe ($K$=4) & 68.05 & 45.15 & 82.47 & 58.27 & \textbf{64.42} & 90.25 & 80.00 & 61.95 & 20.32 & 32.38 & 60.33\\
    X-MoRe ($K$=8) & 69.12 & 44.90 & 83.98 & 59.70 & 64.21 & \textbf{90.37} & \textbf{80.16} & \textbf{62.74} & 20.64 & \textbf{33.76} & 60.96\\
    X-MoRe ($K$=16) & \textbf{69.78} & \textbf{45.17} & 84.96 & \textbf{60.66} & 63.57 & 90.10 & 79.52 & 62.61 & 21.14 & 32.94 & \textbf{61.04}\\
    X-MoRe ($K$=32) & 68.39 & 45.43 & 85.45 & 59.98 & 62.67 & 90.30 & 78.51 & 62.12 & \textbf{21.49} & 30.69 & 60.50\\
    X-MoRe ($K$=64) & 66.60 & 44.62 & \textbf{85.82} & 58.76 & 61.63 & 89.66 & 77.13 & 61.40 & 20.13 & 29.16 & 59.49\\
    \midrule
    % CoOp & 61.55 & 36.94 & 86.75 & 55.38 & 58.74 & 86.61 & 75.59 & 58.19 & 15.18 & 25.75 & 56.07\\
    % TPT & 62.73 & 41.49 & 84.68 & 58.34 & 60.11 & 86.94 & 74.85 & 61.34 & 17.49 & 28.48 & 57.64 \\
    % X-MoRe(with init) & 67.24 & 38.65 & 82.75 & 61.46 & 61.19 & 91.76 & 79.72 & 61.60 & 21.75 & 37.63 & 60.38  \\
    % \midrule
    % \midrule
    CLIP-ViT-B/16$^{\dagger}$ & 67.44 & 44.27 & 88.25 & 65.48 & 65.13 & 93.35 & 83.65 & 62.59 & 23.67 & 42.01 & 63.58 \\
    Caption Ensemble & 61.39 & 36.05 & 60.59 & 44.84 & 51.69 & 85.40 & 71.64 & 49.61 & 20.25 & 33.32 & 51.48\\
    CALIP & 67.64 & 44.44 & 87.82 & 65.80 & 64.05 & 93.27 & 82.76 & 62.52 & 24.12 & 42.27 & 63.47\\

    TPT$^{\dagger}$ & 68.98 & \textbf{47.75}& 87.79 & 66.87 & \textbf{68.04} & \textbf{94.16} & \textbf{84.67} & \textbf{65.50} & 24.78 & 42.44 & 65.10 \\
    X-MoRe ($K$=2) & 68.78 & 46.99 & 81.11 & 62.50 & 66.18 & 93.05 & 83.09 & 62.92 & 24.18 & 40.42 & 62.92\\
    X-MoRe ($K$=4) & 70.55 & 47.95 & 84.59 & 65.30 & 66.51 & 93.62 & 84.44 & 64.33 & 25.34 & 42.53 & 64.52\\
    X-MoRe ($K$=8) & 71.65 & 47.73 & 86.42 & 66.74 & 66.83 & 93.90 & 84.56 & 65.07 & 25.20 & 44.72 & 65.28\\
    X-MoRe ($K$=16) & \textbf{71.65} & 47.36 & 87.61 & \textbf{67.35} & 66.56 & 93.91 & 84.54 & 65.32 & \textbf{25.74} & \textbf{45.81} & \textbf{65.57}\\
    X-MoRe ($K$=32) & 70.78 & 47.18 & 88.23 & 67.07 & 65.87 & 94.00  & 82.24 & 65.21 & 25.48 & 45.61 & 65.37 \\
    X-MoRe ($K$=64) & 68.79 & 46.34 & \textbf{89.01} & 65.91 & 65.46 & 93.75 & 83.88 & 64.85 & 24.28 & 45.38 & 64.77 \\
    % \midrule
    % CoOp & 67.64 & 42.79 & 89.29 & 62.74 & 65.69 & 93.63 & 83.26 & 63.82 & 18.06 & 38.57 & 62.54 \\
    % TPT & 69.27 & 46.57 & 87.00 & 66.51 & 67.67 & 93.79 & 84.70 & 65.07 & 23.10 & 43.05 & 64.67 \\
    % X-MoRe(with init) & 71.38 & 45.33 & 87.49 & 65.01 & 67.01 & 91.72 & 83.54 & 64.85 & 21.93 & 39.49 & 63.77 \\
    \bottomrule
    \end{tabular}
    \caption{Performance across different number of captions used in zero-shot classification benchmark datasets. $^{\dagger}$ performances are from \citet{shu2022test}.}
    \label{tab:appendix_variousK_finegrained}
\end{table*}

\begin{table*}[h]
\small
\centering
    \begin{tabular}{l|ccccc|cc}
    \toprule
    Method & ImageNet & ImageNet-A & ImageNet-V2 & ImageNet-R & ImageNet-Sketch & Avg. & Variants Avg. \\
    \midrule
    CLIP-RN50$^{\dagger}$ & 58.16 & 21.83 & 51.41 & 56.15 & 33.37 & 44.18 & 40.69 \\
    Caption Ensemble & 47.21 & 21.47 & 39.26 & 46.06 & 28.85 & 36.57 & 33.91\\
    CALIP  & 58.21 & 21.67 & 51.44 & 55.96 & 33.30 & 44.12 & 40.59\\
    TPT$^{\dagger}$ & 60.74 & 26.67 & 54.70 & 59.11 & 35.09 & 47.26 & 43.89 \\
    X-MoRe (K=2) & 60.22 & 29.03 & 52.47 & 62.20 & 40.47 & 48.88 & 43.54\\
    X-MoRe (K=4) & 61.81 & \textbf{29.11} & 54.29 & \textbf{63.16} & 41.40 & 49.95 & 46.99\\
    X-MoRe (K=8) & 62.68 & 28.42 & 55.03 & 63.08 & \textbf{41.46} & \textbf{50.13} & \textbf{47.00}\\
    X-MoRe (K=16) & \textbf{62.71} & 26.49 & \textbf{55.25} & 62.21 & 40.41 & 49.41 & 46.09\\
    X-MoRe (K=32) & 62.19 & 25.80 & 54.99 & 61.20 & 39.19 & 48.67 & 45.30 \\
    X-MoRe (K=64) & 61.12 & 25.22 & 53.87 & 59.84 & 37.64 & 47.54 & 44.14\\ 
    % \midrule
    % CoOp & 63.52 & 23.12 & 55.68 & 56.56 & 34.55 & 46.69 & 42.48\\
    % TPT & 60.74 & 26.67 & 54.70 & 59.11 & 35.09 & 47.26 & 43.89 \\
    % X-MoRe (with init) & 65.82 & 28.16 & 58.08 & 62.22 & 41.33 & 51.12 & \textbf{47.45} \\
    % \midrule
    \midrule
    CLIP-ViT-B/16$^{\dagger}$ & 66.73 & 47.87 & 60.86 & 73.98 & 46.09 & 59.11 & 57.20 \\
    Caption Ensemble & 47.11 & 22.62 & 39.64 & 47.84 & 29.34 & 37.31 & 34.86 \\
    CALIP & 66.74 & 47.76 & 60.76 & 73.99 & 46.12 & 59.07 & 57.16 \\
    TPT$^{\dagger}$ & \textbf{68.98} & \textbf{54.77} & \textbf{63.45} & \textbf{77.06} & \textbf{47.94} & \textbf{62.44} & \textbf{60.81} \\
    X-MoRe ($K$=2) & 63.72 & 44.63 & 56.71 & 71.91 & 45.45 & 56.48 & 54.68\\
    X-MoRe ($K$=4) & 65.89 & 46.20 & 58.32 & 73.16 & 46.73 & 58.06 & 56.10\\
    X-MoRe ($K$=8) & 66.65 & 46.76 & 59.50 & 73.71 & 47.00 & 58.72 & 56.74\\
    X-MoRe ($K$=16) & 67.01 & 46.56 & 59.87 & 73.60 & 46.61 & 58.73 & 56.66 \\
    X-MoRe ($K$=32) & 67.01 & 46.20 & 59.89 & 73.52 & 46.25 & 58.57 & 56.47\\
    X-MoRe ($K$=64) & 66.77 & 45.87 & 59.77 & 73.17 & 45.77 & 58.27 & 56.15\\ 
    % \midrule
    % CoOp & 71.59 & 50.08 & 64.43 & 74.63 & 47.45 & 61.64 & 59.15\\
    % TPT & 68.98 & 54.77 & 63.45 & 77.06 & 47.94 & 62.44 & \textbf{60.81} \\
    % X-MoRe (with init) & 70.56 & 48.65 & 62.66 & 74.03 & 46.83 & 60.33 & 58.04\\
    \bottomrule
    \end{tabular}
    \caption{Performance across different number of retrieved captions used on ImageNet and its variants. $^{\dagger}$ performances are from \citet{shu2022test}.}
    \label{tab:appendix_variousK_imagenet}
\end{table*}

%  with pretrained initialization by CoOp \cite{zhou2022learning}

\subsection{Zero-shot with Fine-tuned Prompt}
In this section, we evaluate the efficacy of our method when combined with fine-tuned initialization obtained from prompt tuning. We aim to understand the interplay between our technique and the initial weight, and how they collectively influence the overall performance. We use four context vectors fine-tuned for 50 epochs with 16 shots per class in ImageNet \cite{deng2009imagenet}, referring to CoOp \cite{zhou2022learning}.

 \begin{table*}[hbt!]
 \small
 \centering
     \begin{tabular}{l|ccccc|cc}
     \toprule
     Method & ImageNet & ImageNet-A & ImageNet-V2 & ImageNet-R & ImageNet-Sketch & Avg. & Variants Avg. \\
     \midrule
     CLIP-RN50 & 58.16 & 21.83 & 51.41 & 56.15 & 33.37 & 44.18 & 40.69 \\
     % Caption Ensemble & & & \\
     % CALIP  & 58.21 & 21.67 & 51.44 & 55.96 & 33.30 & 44.12 & 40.59\\
     % \midrule
     % TPT & 60.74 & 26.67 & 54.70 & 59.11 & 35.09 & 47.26 & 43.89 \\
     X-MoRe ($K$=2) & 63.20 & 29.93 & 54.86 & 62.14 & 41.23 & 50.27 & 47.04\\
     X-MoRe ($K$=4) & 65.01 & 29.79 & 56.72 & 63.13 & 42.13 & 51.36 & 47.94\\
     X-MoRe ($K$=8) & 65.78 & 29.08 & 57.87 & 62.95 & 42.11 & 51.56 & \textbf{48.00}\\
     X-MoRe ($K$=16) & 65.82 & 28.16 & 58.08 & 62.22 & 41.33 & 51.12 & 47.45 \\
     X-MoRe ($K$=32) & 65.32 & 27.09 & 57.57 & 61.19 & 39.75 & 50.18 & 46.40 \\
     X-MoRe ($K$=64) & 64.41 & 26.05 & 56.54 & 60.03 & 38.28 & 49.06 & 45.22\\
     \midrule
     CLIP-ViT-B/16 & 66.73 & 47.87 & 60.86 & 73.98 & 46.09 & 59.11 & 57.20 \\
     % Caption Ensemble & & & &\\
     % CALIP & 66.74 & 47.76 & 60.76 & 73.99 & 46.12 & 59.07 & 57.16 \\
     % \midrule
     % TPT & 68.98 & 54.77 & 63.45 & 77.06 & 47.94 & 62.44 & 60.81 \\
     X-MoRe ($K$=2) & 66.96 & 47.09 & 59.34 & 72.36 & 45.29 & 58.21 & 56.02\\
     X-MoRe ($K$=4) & 69.29 & 48.38 & 61.29 & 73.67 & 46.72 & 59.87 & 57.52\\
     X-MoRe ($K$=8) & 70.13 & 48.16 & 62.09 & 74.10 & 47.00 & 60.30 & 57.84\\
     X-MoRe ($K$=16) & 70.56 & 48.65 & 62.66 & 74.03 & 46.83 & 60.33 & \textbf{58.04}\\
     X-MoRe ($K$=32) & 70.65 & 48.52 & 62.93 & 73.94 & 46.63 & 60.53 & 58.01\\
     X-MoRe ($K$=64) & 70.49 & 48.18 & 63.07 & 73.81 & 46.12 & 60.33 & 57.80\\ 
    
     \bottomrule
     \end{tabular}
     \caption{Performance with fine-tuned initialization by CoOp \citep{zhou2022learning} with ImageNet \citep{deng2009imagenet} }
     \label{tab:pretrained_init}
 \end{table*}

In Table~\ref{tab:pretrained_init}, our zero-shot method with pre-trained initialization from ImageNet \cite{deng2009imagenet} shows improvements compared to class templates, e.g., ``a photo of a [CLS]''.

\subsection{Effect of the Number of Candidate Pairs ($N$)}
 \begin{table*}[hbt!]
 \small
 \centering
     \begin{tabular}{l|ccccc|cc}
     \toprule
     Method & ImageNet & ImageNet-A & ImageNet-V2 & ImageNet-R & ImageNet-Sketch & Avg. & Variants Avg. \\
     \midrule
     CLIP-RN50 & 58.16 & 21.83 & 51.41 & 56.15 & 33.37 & 44.18 & 40.69 \\
     X-MoRe ($N$=128) & 62.71 & 26.49 & 55.25 & 62.21 & 40.41 & 49.41 & 46.09 \\
     X-MoRe ($N$=256) & 62.84 & 28.48 & 55.04 & 62.92 & 40.82 & \textbf{50.02} & \textbf{46.82}\\
     \midrule
     CLIP-ViT-B/16 & 66.73 & 47.87 & 60.86 & 73.98 & 46.09 & \textbf{59.11} & \textbf{57.20} \\
     X-MoRe ($N$=128) & 67.01 & 46.56 & 59.87 & 73.60 & 46.61 & 58.73 & 56.66\\
     X-MoRe ($N$=256) & 66.92 & 46.87 & 59.35 & 73.70 & 46.70 & 58.71 & 56.66 \\
    
     \bottomrule
     \end{tabular}
     \caption{Performance under ImageNet and the variants, where $K=16$ \cite{deng2009imagenet} }
     \label{tab:appendix_N}
 \end{table*}
In this section, we check the effectiveness of increasing number of candidate pairs, i.e $N$, of image-based retrieval. As shown in Table \ref{tab:appendix_N}, we doubled the number of retrievals from 128 to 256 and evaluate on ImageNet and its variants. It is interesting to note that the accuracy improves when retrieving captions is beneficial than baseline CLIP. In other words, when the performance gap exists between the captions and images, increasing the size $N$ is not helpful.  
Thus, the results show that the accuracy improves when retrieving more captions is beneficial, although there is a trade-off between the performance and retrieval cost.

% \subsection{Ranking correlation between Image-based Retrieval and Text-based Fine-retrieval}
% In this section, we measure the correlation between orders of captions retrieved based on image modality and text modality. The purpose is to confirm the importance of text-based fine-retrieval which directly measures the similarity between input query and corresponding captions, instead of images in the external dataset.
% As shown in Table ~, the ranking corre
% In summary, 

\subsection{Effect of the Order of Test Samples}
We run TPT multiple times using three different random seeds and report the average accuracy. The randomness of \texttt{X-MoRe} only comes from random shuffling of test data. To offer a more comprehensive understanding of the variability in our experiments, we provide standard deviation in \ref{tab:appendix_error_bars_fs} and \ref{tab:appendix_error_bars_imagenet} for the results in Table 1 and Table 2 in the main paper.

\begin{table*}[h]
\scriptsize
\centering
\setlength{\tabcolsep}{2pt}
    \begin{tabular}{l|cccccccccc|c}
    \toprule
    Method & Flower102 & DTD & Pets & Cars & UCF101 & Caltech101 & Food101 & SUN397 & Aircraft & EuroSAT & Avg. \\
    \midrule
    X-MoRe (RN50) & 69.78$\pm0.07$ & 45.17$\pm0.03$ & 84.96$\pm0.03$ & 60.66$\pm0.02$ & 63.57$\pm0.02$ & 90.10$\pm0.03$ & 79.52$\pm0.01$ & 62.61$\pm0.01$ & 21.14$\pm0.03$& 32.94$\pm0.01$ & 61.04$\pm0.21$\\
    \midrule
    X-MoRe (ViT-B/16) & 71.65$\pm0.02$& 47.36$\pm0.03 $ & 87.61$\pm0.01$ & 67.35$\pm0.01$ & 66.56$\pm0.13$ & 93.91$\pm0.00$ & 84.54$\pm0.00$ & 65.32$\pm0.01$ & 25.74$\pm0.00$ & 45.81$\pm0.02$ & 65.57$\pm0.20$\\
    \bottomrule
    \end{tabular}
     \caption{Accuracy with standard deviation according to the three different random seeds on zero-shot classification datasets, when $K=16$}
     \label{tab:appendix_error_bars_fs}

\end{table*}
 \begin{table*}[hbt!]
 \small
 \centering
     \begin{tabular}{lccccccc}
     \toprule
     Method & ImageNet & ImageNet-A & ImageNet-V2 & ImageNet-R & ImageNet-Sketch & Avg. & Variants Avg. \\
     \midrule
     % CLIP-RN50 & 58.16 & 21.83 & 51.41 & 56.15 & 33.37 & 44.18 & 40.69 \\
     X-MoRe (RN50) & 62.71$\pm0.00$ & 26.49$\pm0.02$ & 55.25$\pm0.00$ & 62.21$\pm0.00$ & 40.41$\pm0.00$ & 49.41$\pm0.00$ & 46.09$\pm0.14$ \\
     \midrule
     % CLIP-ViT-B/16 & 66.73 & 47.87 & 60.86 & 73.98 & 46.09 & \textbf{59.11} & \textbf{57.20} \\
     X-MoRe (ViT-B/16) & 67.01$\pm0.00$& 46.56$\pm0.00$ & 59.87$\pm0.00$ & 73.60$\pm0.00$ & 46.61$\pm0.00$ & 58.73$\pm0.00$ & 56.66$\pm0.11$\\
     \bottomrule
     \end{tabular}
     \caption{Accuracy with standard deviation according to the three different random seeds on domain generalization datasets, when $K=16$.}
     \label{tab:appendix_error_bars_imagenet}
 \end{table*}
